# Supplementary material for: UASTHN: Uncertainty-Aware Deep Homography Estimation for UAV Satellite-Thermal Geo-localization
Source: arXiv:2502.01035 source file (2025-02-24)
Supplement: Supplementary file 1 [file 7_appendix.tex]

In the Appendix, we present the supplementary information and results for a better understanding the our work. Section~\ref{imp} presents the implementation details including hyperparameters configuration. Section~\ref{grid} details the grid sampling for CropTTA. Section~\ref{data} shows more details about the dataset. Section~\ref{inference} shows statistics about the inference time of our methods. Section~\ref{histogram} shows the histogram of MACE for our methods. Section~\ref{extended_ab} shows the extended plot of the ablation study for lower success rates.

\subsection{Implementation Details}\label{imp}
For our implementation, we set iteration numbers of the iterative homography networks $K_1=6$ and the iteration number of the second-stage model $K_2=6$. Resizing width $W_R$ is set to $256$. Decay factor $\gamma$ is set to 0.85. For the training process, we first train the model $F_H$ without CropTTA for $200,000$ iterations. Then we finetune the model with CropTTA for $200,000$ iterations. For the two-stage methods, We use bounding box augmentation~\cite{STHN}, which randomly perturbs the first-stage results by 64 pixels for each of the four corners. During the evaluation of two-stage models, the width of the bounding box $W_B$ is instead consistently expanded by 64 pixels (32 pixels on each side). If not specified, all uncertainty estimation methods are evaluated with 5 samples. The homography networks are trained using the AdamW optimizer~\cite{loshchilov2017decoupled}, with a linear decay scheduler and warmup at a maximum learning rate of $1\times10^{-4}$.

\subsection{Details of CropTTA Sampling Methods}\label{grid}
Fig.\ref{croptta_method} illustrates the impact of various crop offsets ($o_c$) on cropped thermal images, showing that larger crop offsets result in smaller crop sizes. It also shows the visual comparison between random and grid sampling for CropTTA.
\begin{figure}[!htb]
\begin{subfigure}[b]{0.33\textwidth}
    \includegraphics[width=\textwidth]{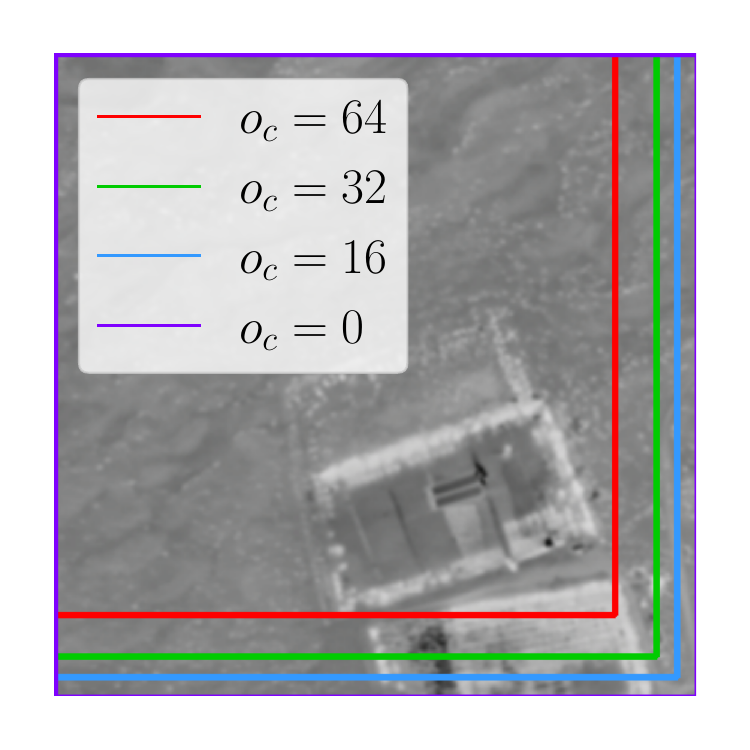}
    \caption{Crop offset}
\end{subfigure}
\begin{subfigure}[b]{0.33\textwidth}
\includegraphics[width=\textwidth]{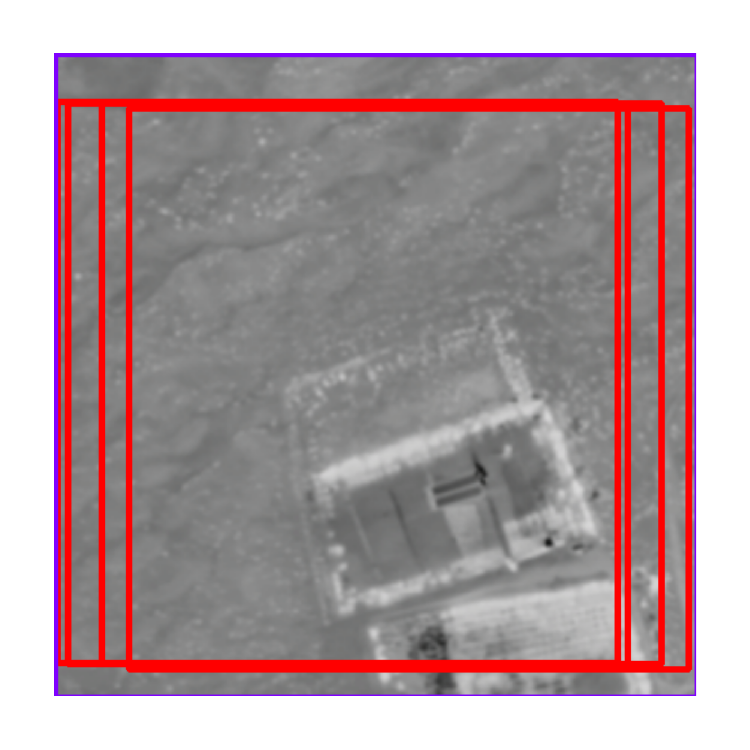}
    \caption{Random sampling}
\end{subfigure}
\begin{subfigure}[b]{0.33\textwidth}
\includegraphics[width=\textwidth]{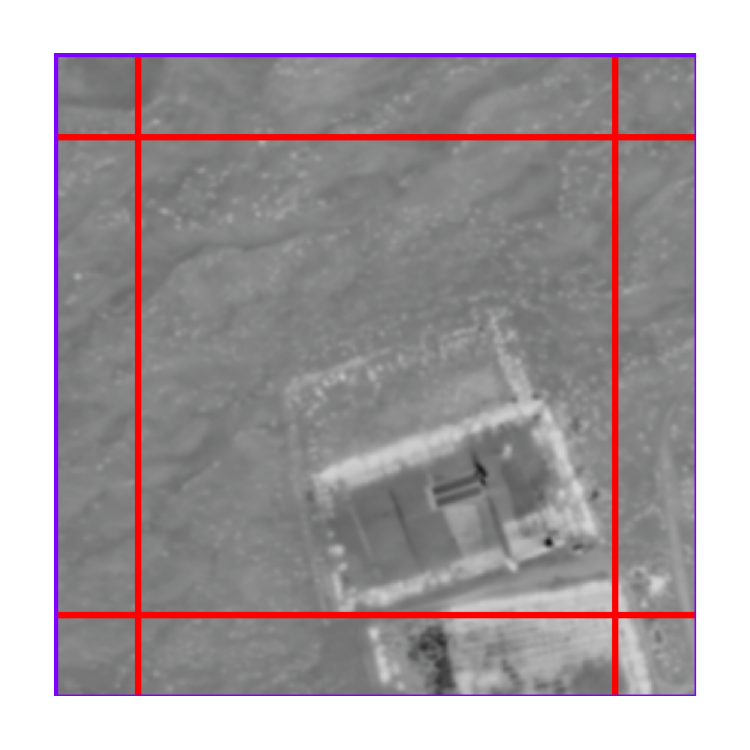}
    \caption{Grid sampling}
\end{subfigure}
    \caption{Visualization of crop offset ($o_c$) and sampling methods for CropTTA. The colored boxes represent cropping regions with different crop offsets.}
    \label{croptta_method}
    \vspace{-15pt}
\end{figure}

\subsection{Dataset Details}\label{data}
For image processing of thermal images, the dataset utilized the Structure-from-Motion (SfM) technique to seamlessly merge the captured thermal image patches from each flight, creating separate maps for significant temperature changes between flights. Following this, the maps were cropped to sample images with a resolution of $512\times512$ pixels and a sampling stride of $35$ pixels. The alignment between satellite and thermal images is based on the aggregated results of the GPS position of the images and manual adjustment. This alignment also ensures a spatial resolution of approximately $1$ pixel per meter for both modalities. Our data assumes that a compass and gimbal are used to north-align the thermal images in practical applications.

\subsection{Inference Time}\label{inference} Table~\ref{time} compares the inference times of different UE methods. The results indicate that CropTTA is more efficient than DE for both one-stage and two-stage methods. Additionally, early stopping helps to reduce the increase in inference time associated with a higher number of samples, highlighting its practicality for real-time TG applications.

\begin{table}
    \centering
    \caption{Comparison of inference time (\si{ms}) for different UE methods with or without early stopping. We evaluate with 5 samples and in an NVIDIA RTX 2080Ti GPU.}
        \resizebox{0.9\textwidth}{!}{
    \begin{tabular}{lccccccccc}
    \toprule
       \multirow{2}{4em}{Early Stopping} & \multicolumn{4}{c}{IHN (one-stage)~\cite{cao2022iterative}}& &\multicolumn{4}{c}{STHN (two-stage)~\cite{STHN}}\\
       \cline{2-5} \cline{7-10}\vspace{-10pt}\\
       & w/o UE & CropTTA & DE & CropTTA + DE & & w/o UE & CropTTA & DE & CropTTA + DE\\
         \midrule
         \xmark & 35.2 & 64.6 & 114.6 & 164.2&  &63.9  &87.0 & 130.2  & 186.0 \\
         \checkmark & - & 54.6 &63.1 & 92.1 & & - &78.2 & 81.9 & 118.6\\
    \bottomrule
    \end{tabular}}
    \vspace{-10pt}
    \label{time}
\end{table}

\subsection{MACE Histogram}\label{histogram} Fig.\ref{hist} presents the histogram of MACE for the CropTTA with STHN two-stage method across different $D_C$. We observe that for larger $D_C$ values ($256~\si{m}$ and $512~\si{m}$), the histogram exhibits a long-tail error distribution. In contrast, for the smaller $D_C$ ($128~\si{m}$), the majority of cases fall below $25~\si{m}$, which is within the expected rejection error threshold. This pattern explains why larger $D_C$ values yield better ROC curves—because the outliers in the long tail are more easily detected at larger $D_C$.

\begin{figure}
    \centering
    \includegraphics[width=0.5\linewidth]{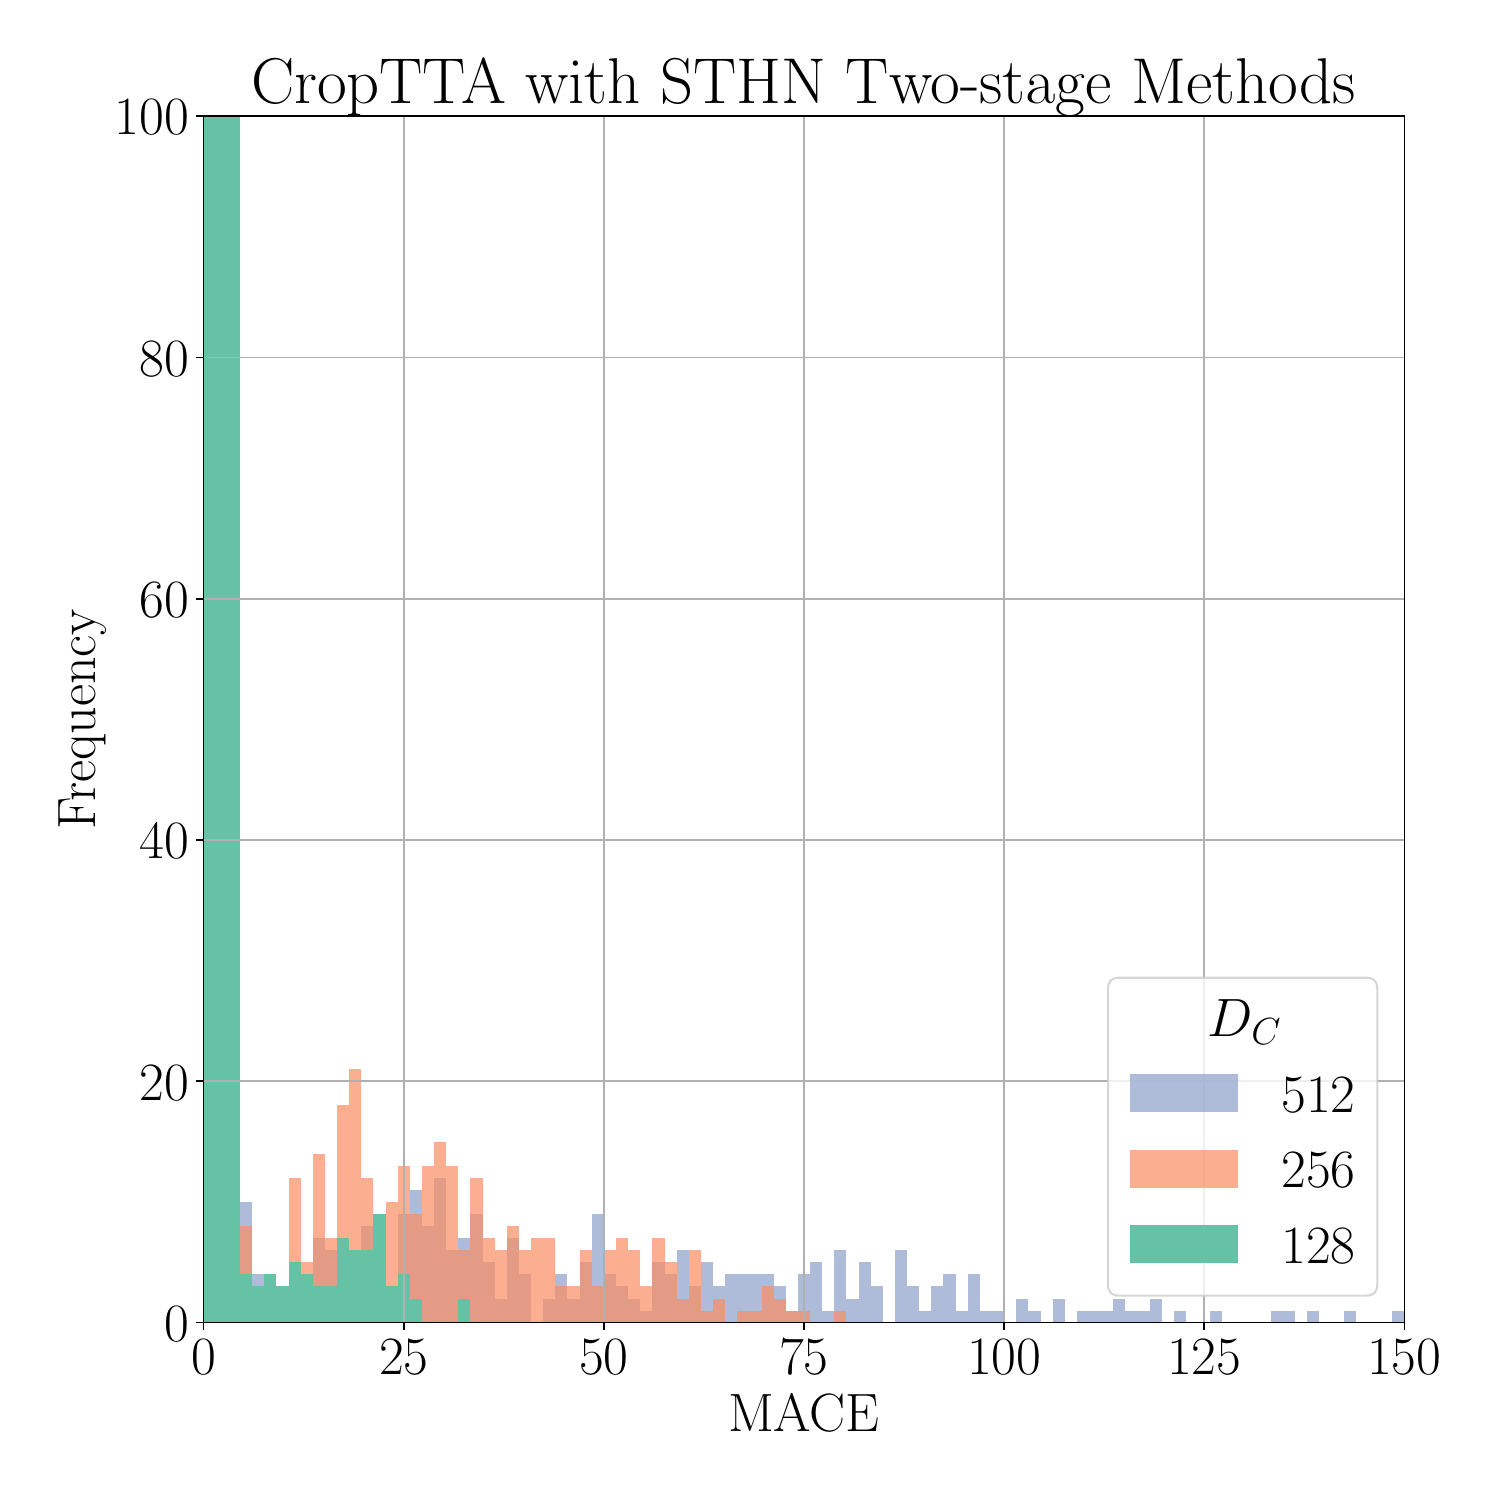}
    \caption{MACE histogram for CropTTA with STHN two-stage methods across different $D_C$}
    \label{hist}
\end{figure}

\subsection{Extended Plots for Ablation Study}\label{extended_ab} Fig.~\ref{extended} presents an extended plot of the ablation study, focusing on success rates between $95\%$ and $50\%$. This comparison for lower success rates reveals trends similar to those observed in Fig.\ref{ablation}.

\begin{figure}[]
\begin{subfigure}[b]{0.33\textwidth}
    \includegraphics[width=\textwidth]{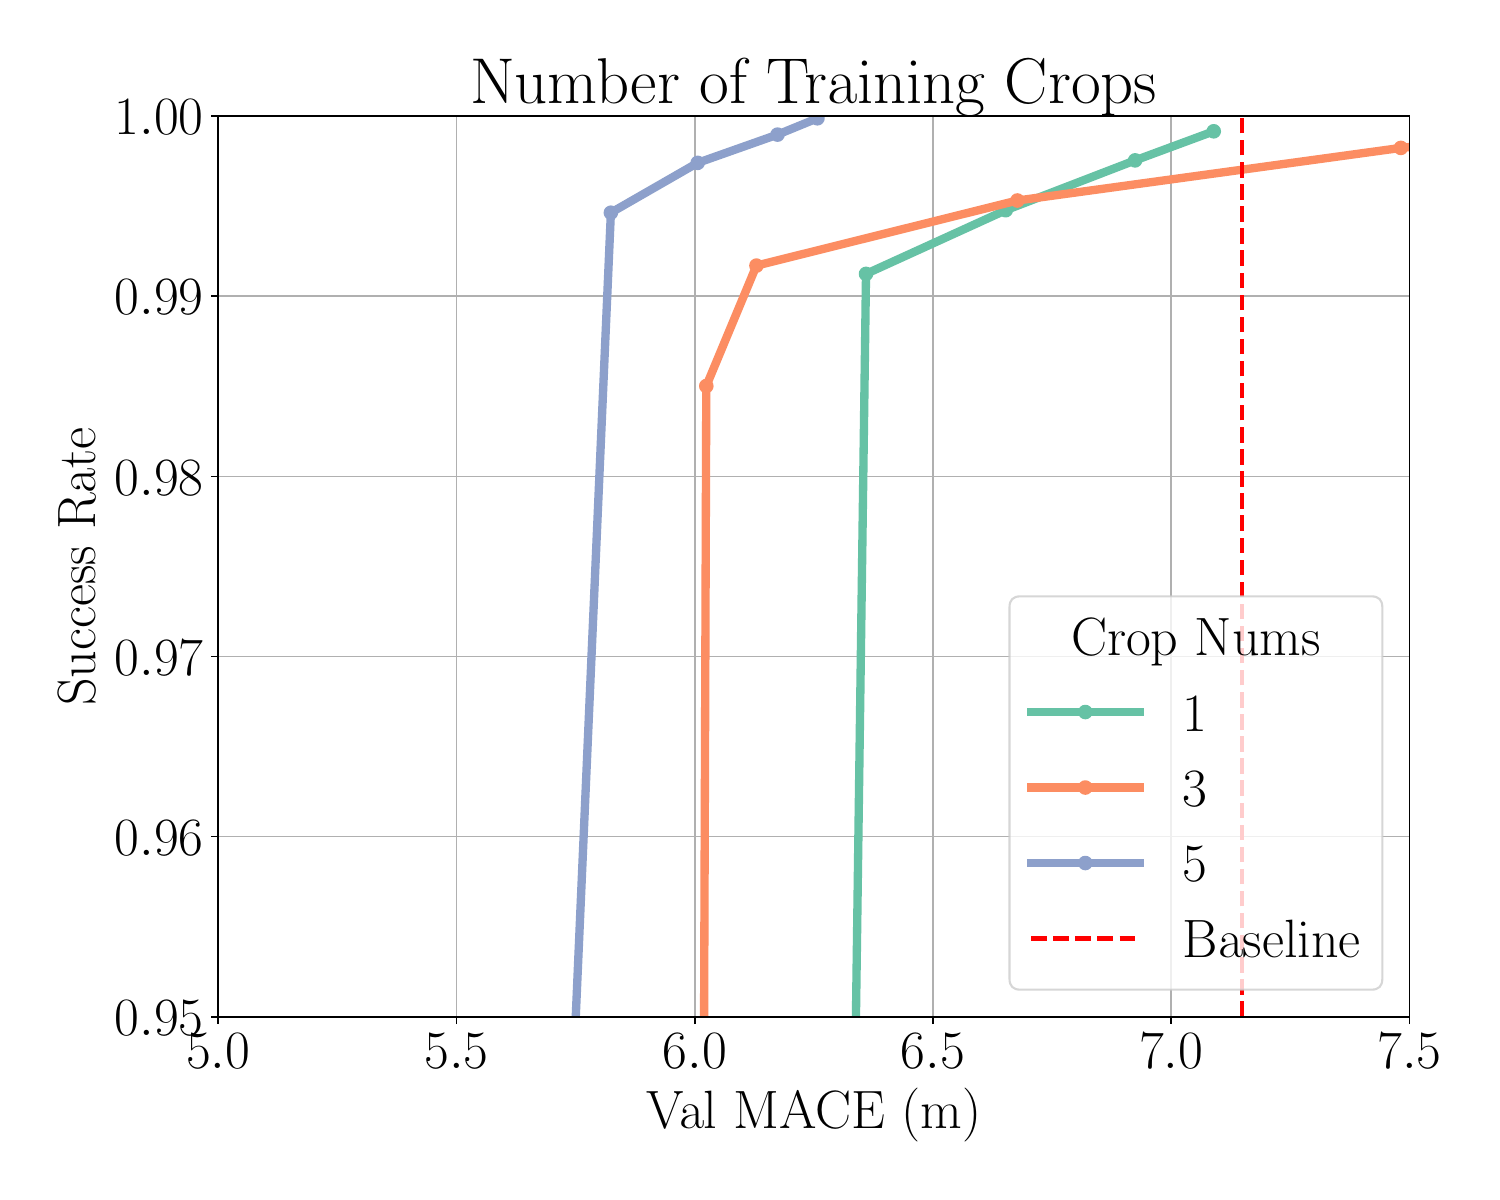}
    \caption{Number of Training Crops}
    \label{mct}
\end{subfigure}
\begin{subfigure}[b]{0.33\textwidth}
    \includegraphics[width=\textwidth]{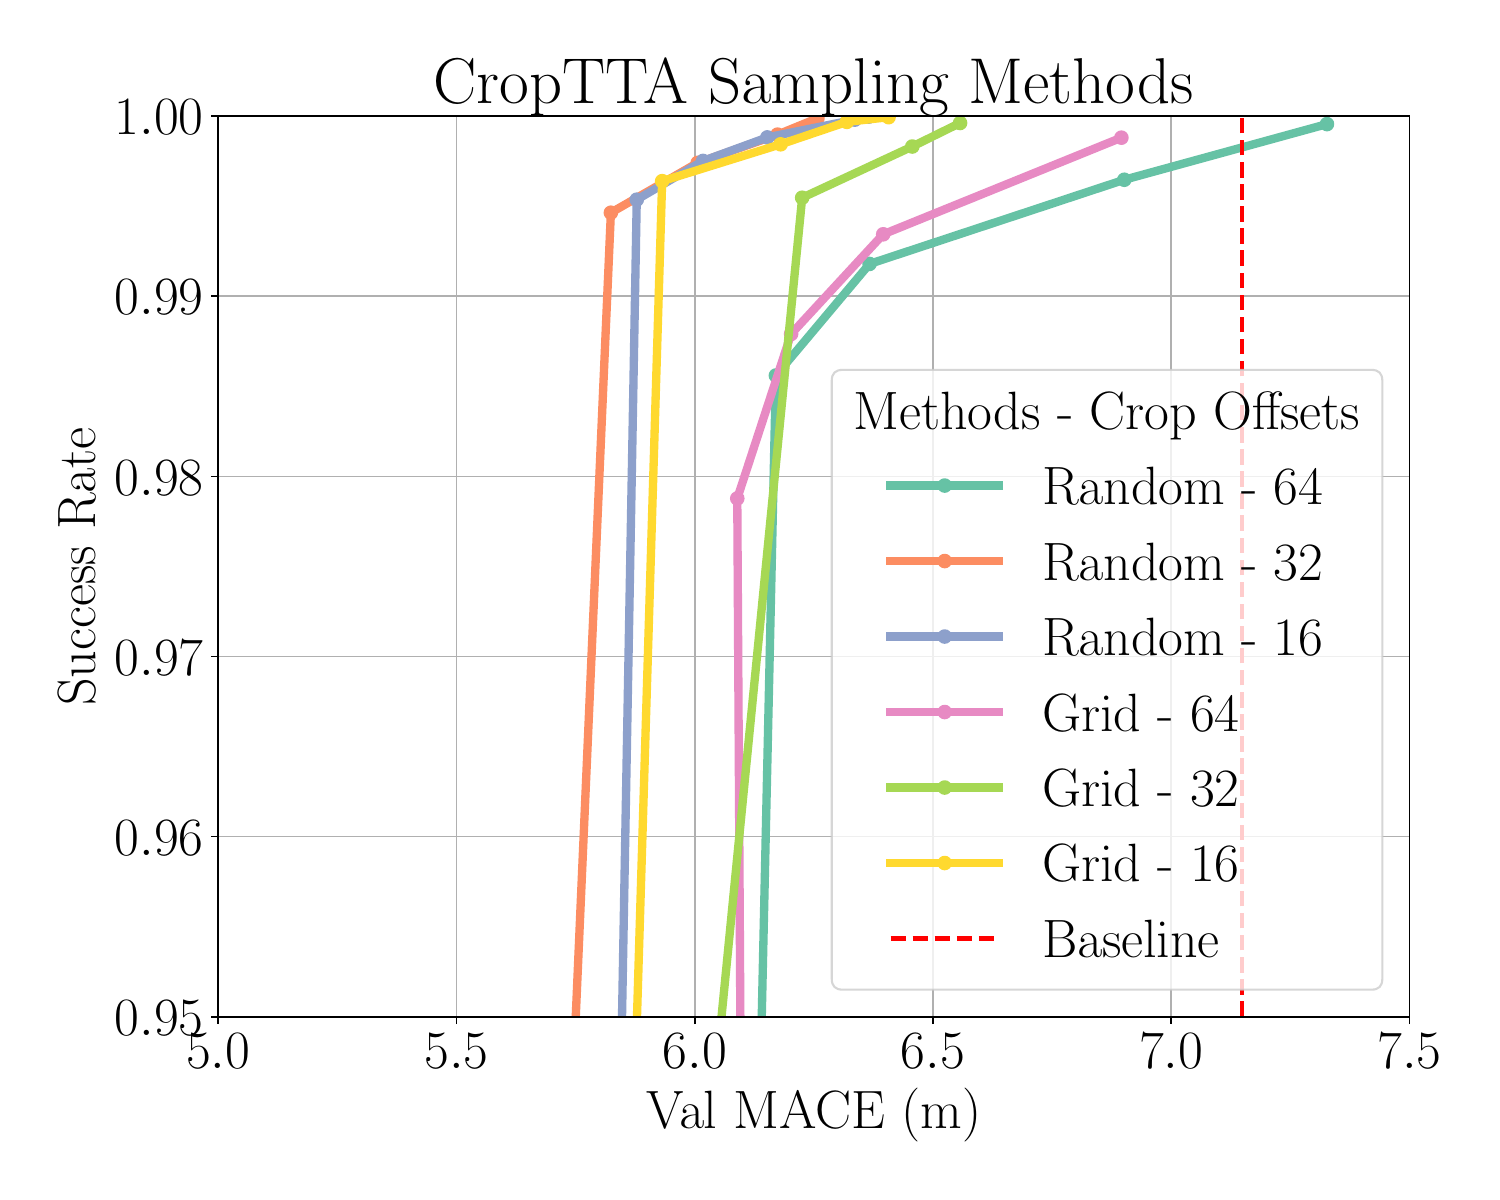}
    \caption{Sampling Methods}
    \label{croptta}
\end{subfigure}
\begin{subfigure}[b]{0.33\textwidth}
    \includegraphics[width=\textwidth]{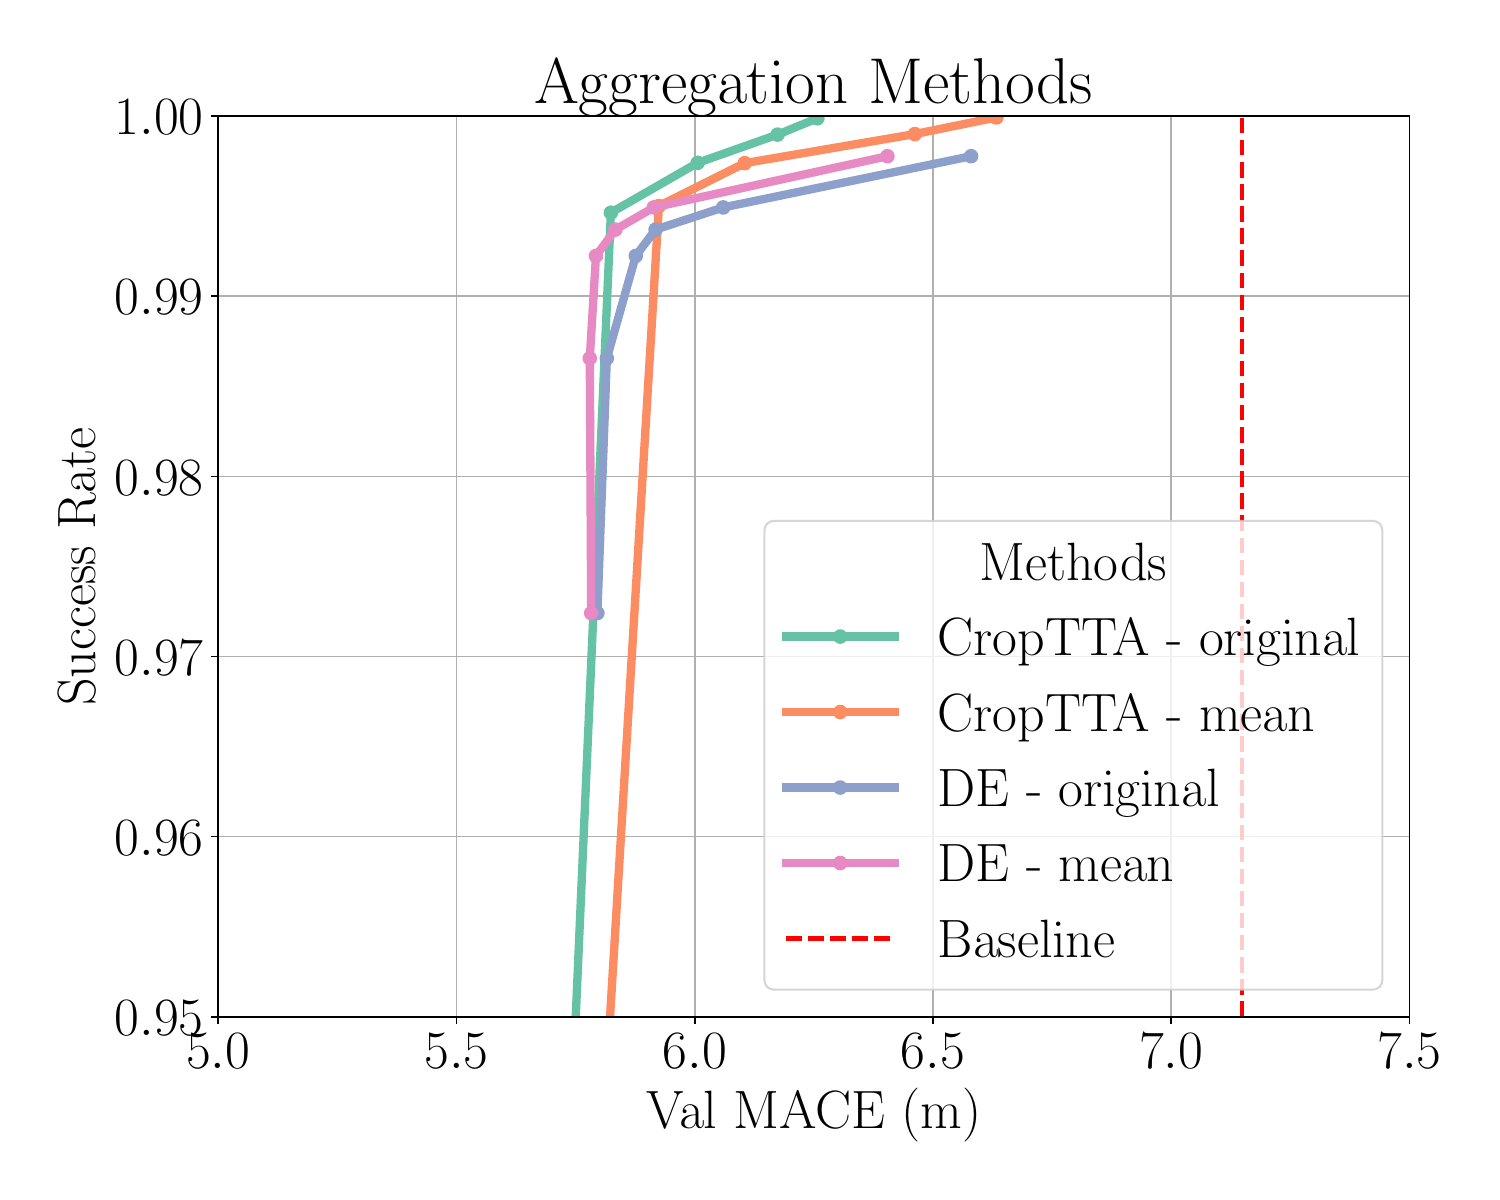}
    \caption{Aggregation Methods}
    \label{agg}
\end{subfigure}
\begin{subfigure}[b]{0.33\textwidth}
    \includegraphics[width=\textwidth]{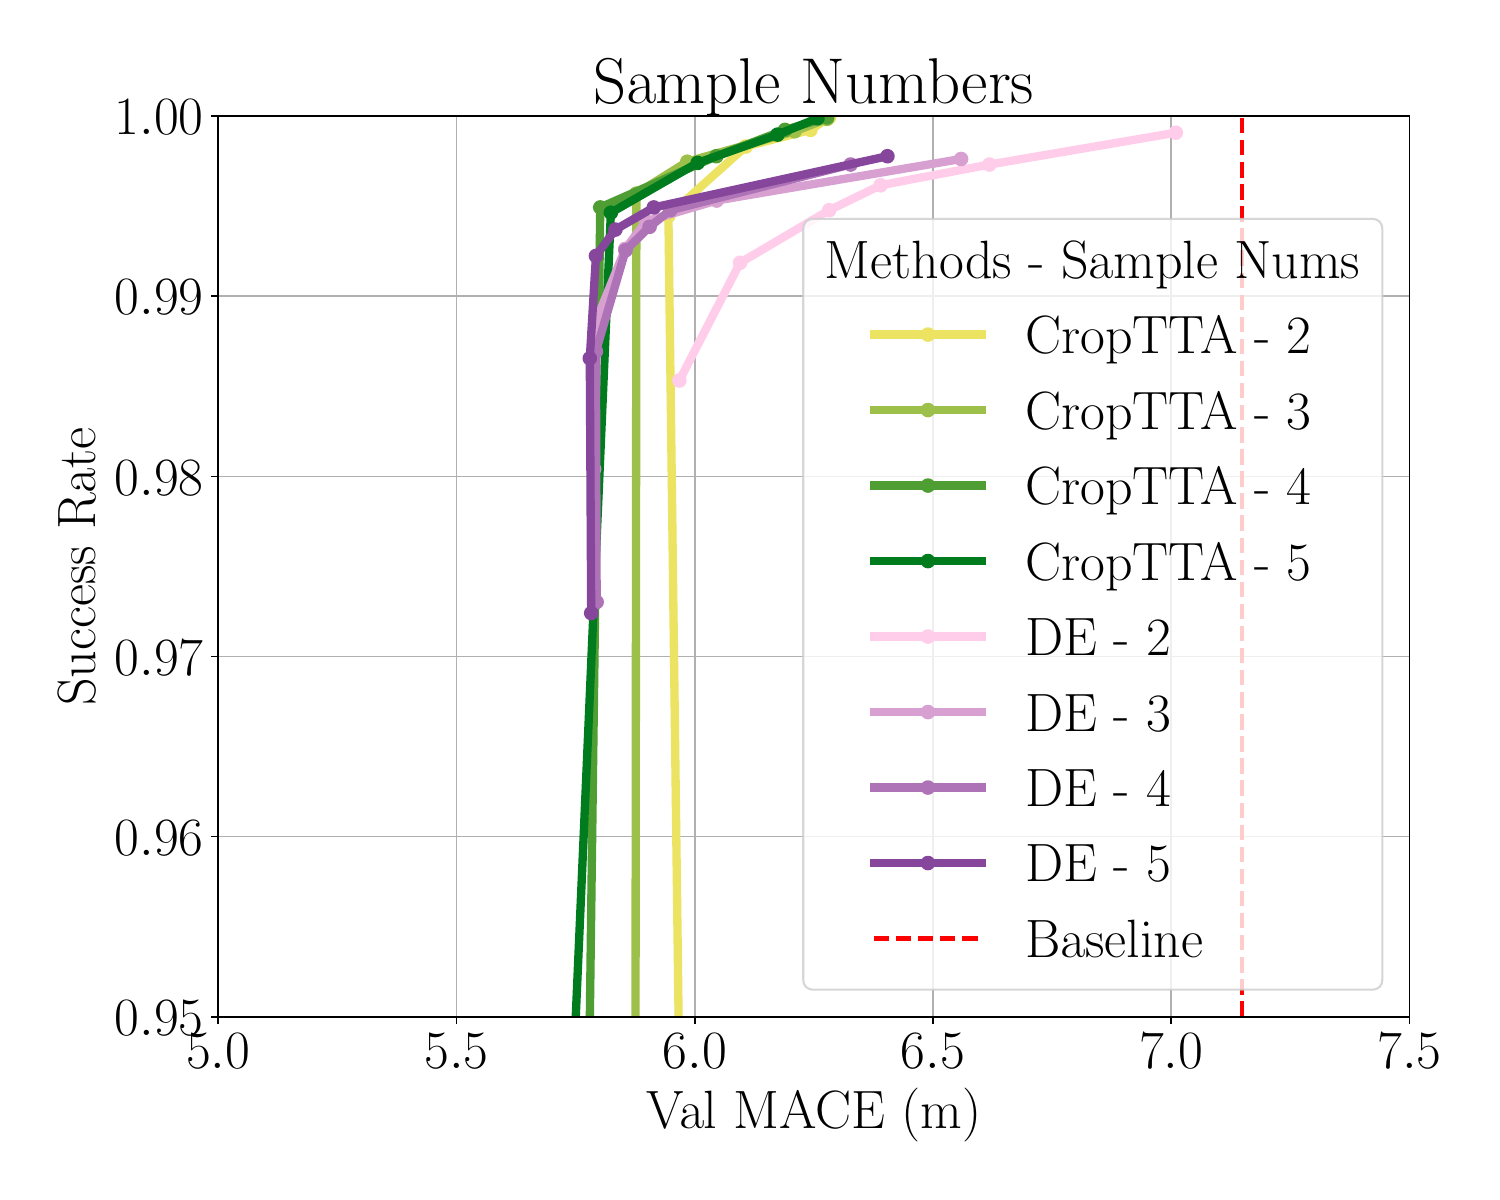}
    \caption{Sample Numbers}
    \label{sample}
\end{subfigure}
\begin{subfigure}[b]{0.33\textwidth}
    \includegraphics[width=\textwidth]{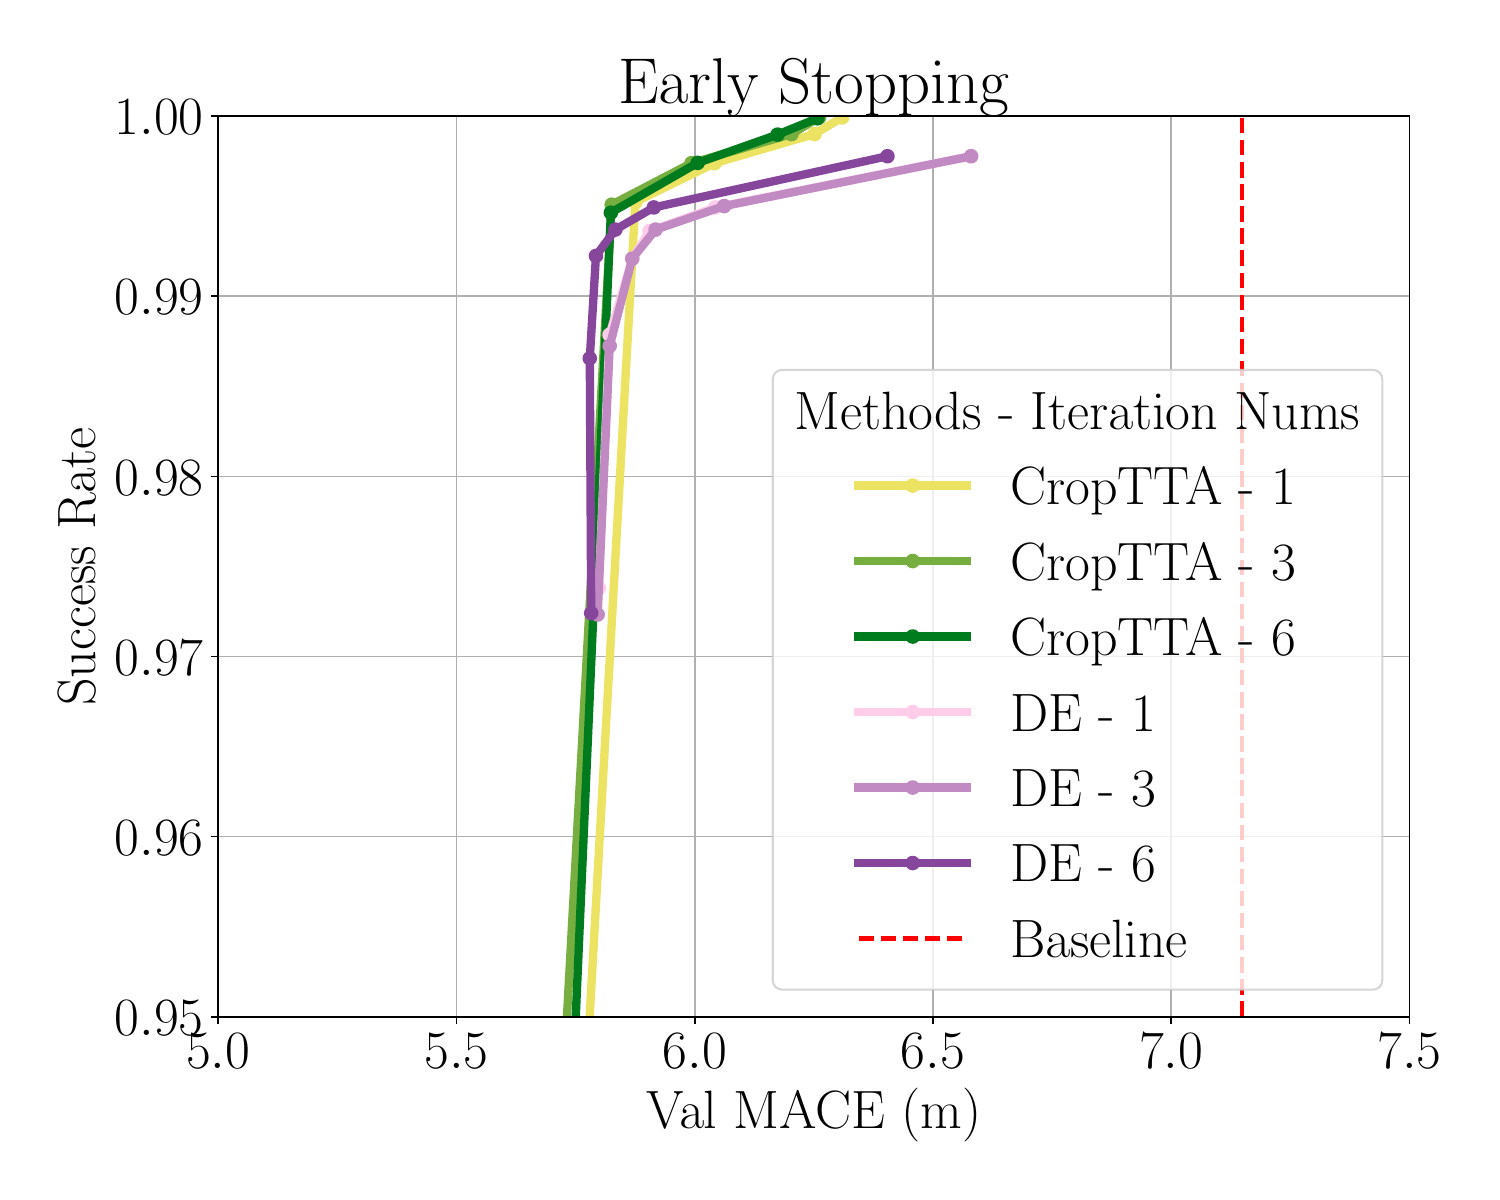}
    \caption{Early Stopping}
    \label{cs}
\end{subfigure}
\begin{subfigure}[b]{0.33\textwidth}
    \includegraphics[width=\textwidth]{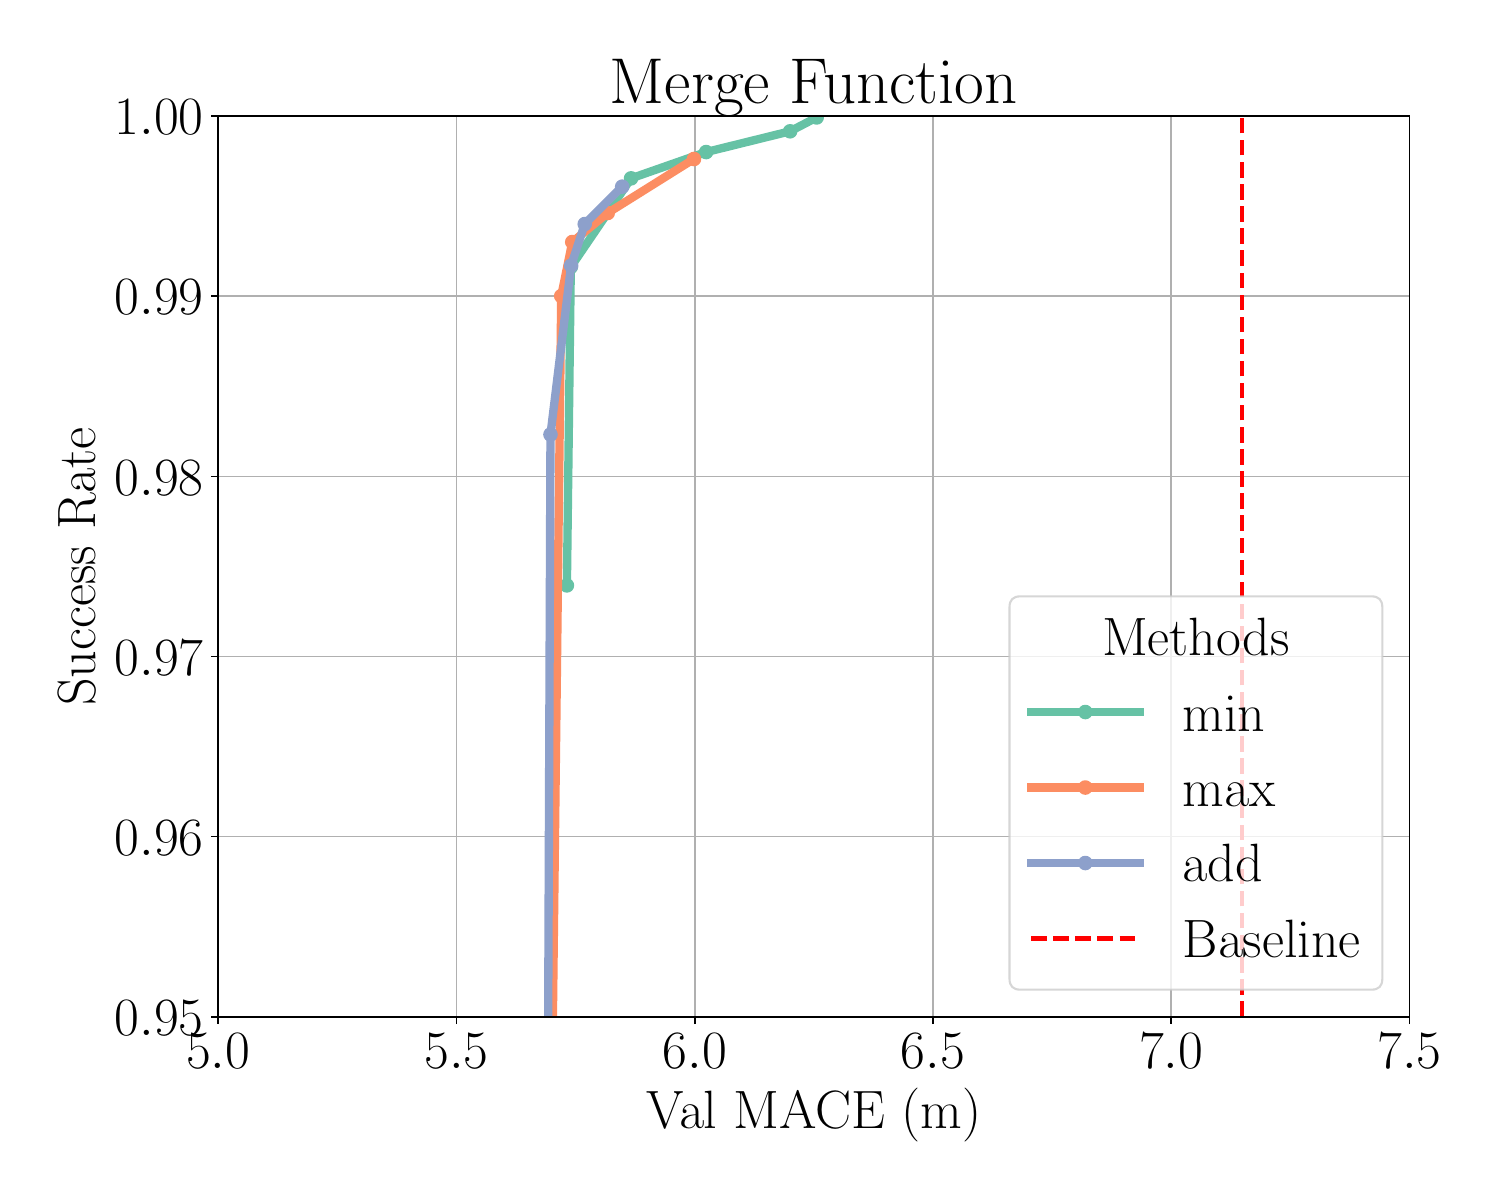}
    \caption{Merge Function}
    \label{merge}
\end{subfigure}
    \caption{Extended plots of Ablation Study. We use success rate and Validation (Val) MACE metrics to ablate the training and evaluation settings. \textit{Baseline} indicates STHN~\cite{STHN} two-stage baseline performance.}
    \label{extended}
    \vspace{-15pt}
\end{figure}
